# Supplementary material for: The universality of electronic friction II: Equivalence of the quantum-classical Liouville equation approach with von Oppen's nonequilibrium Green's function methods out of equilibrium
Source: arXiv:1801.06108 ancillary file (2018-01-19)
Supplement: Supplementary file 1 [file SM7.pdf]

# The universality of electronic friction II: Equivalence of the quantum-classical Liouville equation approach with von Oppen's nonequilibrium Green's function methods out of equilibrium (Supplemental Material)

Wenjie Dou and Joseph E. Subotnik
*Department of Chemistry, University of Pennsylvania, Philadelphia, Pennsylvania 19104, USA*

In this Supplemental Material (SM), we will evaluate the nonequilibrium electronic friction in the non-Condon approximation,

$$\gamma_{\mu\nu} = \hbar \int \frac{d\epsilon}{2\pi} Tr_m \left(\partial_\mu \mathcal{H} \partial_\epsilon \mathcal{G}^R(\epsilon) \partial_\nu \mathcal{H} \mathcal{G}^<(\epsilon)\right) + h.c. \tag{34}$$

Here, h.c. denotes the Hermitian conjugate. We first evaluate $Tr_m \left(\partial_\mu \mathcal{H} \partial_\epsilon \mathcal{G}^R(\epsilon) \partial_\nu \mathcal{H} \mathcal{G}^<(\epsilon)\right)$. For the quadratic electronic Hamiltonian in Eqs. 21-24, we have the following terms:

$$Tr_m \left(\partial_\mu \mathcal{H} \partial_\epsilon \mathcal{G}^R(\epsilon) \partial_\nu \mathcal{H} \mathcal{G}^<(\epsilon)\right) \tag{35}$$

$$= \sum_{mnm'n'} \partial_\mu h_{mn} \partial_\epsilon G^R_{nm'} \partial_\nu h_{m'n'} G^<_{n'm} \tag{36}$$

$$+ \sum_{mnm',k\alpha} \partial_\mu h_{mn} \partial_\epsilon G^R_{nm'} \partial_\nu V_{m',k\alpha} \mathcal{G}^<_{k\alpha,m} \tag{37}$$

$$+ \sum_{mnm',k\alpha} \partial_\mu h_{mn} \partial_\epsilon \mathcal{G}^R_{n,k\alpha} \partial_\nu V_{k\alpha,m'} G^<_{m',m} \tag{38}$$

$$+ \sum_{mnm',k\alpha} \partial_\mu V_{m,k\alpha} \partial_\epsilon \mathcal{G}^R_{k\alpha,m'} \partial_\nu h_{m',n} G^<_{n,m} \tag{39}$$

$$+ \sum_{mnm',k\alpha} \partial_\mu V_{k\alpha,n} \partial_\epsilon G^R_{n,m'} \partial_\nu h_{m',m} \mathcal{G}^<_{m,k\alpha} \tag{40}$$

$$+ \sum_{mn,k'\alpha',k\alpha} \partial_\mu V_{k\alpha,n} \partial_\epsilon \mathcal{G}^R_{n,k'\alpha'} \partial_\nu V_{k'\alpha',m} \mathcal{G}^<_{m,k\alpha} \tag{41}$$

$$+ \sum_{mn,k'\alpha',k\alpha} \partial_\mu V_{k\alpha,n} \partial_\epsilon G^R_{nm} \partial_\nu V_{m,k'\alpha'} \mathcal{G}^<_{k'\alpha',k\alpha} \tag{42}$$

$$+ \sum_{mn,k'\alpha',k\alpha} \partial_\mu V_{n,k\alpha} \partial_\epsilon \mathcal{G}^R_{k\alpha,m} \partial_\nu V_{m,k'\alpha'} \mathcal{G}^<_{k'\alpha',n} \tag{43}$$

$$+ \sum_{mn,k'\alpha',k\alpha} \partial_\mu V_{n,k\alpha,} \partial_\epsilon \mathcal{G}^R_{k\alpha,k'\alpha'} \partial_\nu V_{k'\alpha',m} G^<_{m,n} \tag{44}$$

To simplify the above equations, we will apply Dyson equations,

$$\mathcal{G}_{m,k\alpha} = \sum_{n'} G_{m,n'} V_{n',k\alpha} g_{k\alpha} \tag{45}$$

$$\mathcal{G}_{k\alpha,m} = \sum_{n'} g_{k\alpha} V_{k\alpha,n'} G_{n',m} \tag{46}$$

$$\mathcal{G}_{k\alpha,k'\alpha'} = g_{k\alpha}\delta_{k\alpha,k'\alpha'} + \sum_{mn} g_{k\alpha} V_{k\alpha,n} G_{n,m} V_{m,k'\alpha'} g_{k'\alpha'} \tag{47}$$

The Dyson equation will be projected onto the retarded (advanced) and lesser Green's functions. For example, Eq. 45 gives us

$$\mathcal{G}^R_{m,k\alpha} = \sum_{n'} G^R_{m,n'} V_{n',k\alpha} g^r_{k\alpha} \tag{48}$$

$$\mathcal{G}^<_{m,k\alpha} = \sum_{n'} G^R_{m,n'} V_{n',k\alpha} g^<_{k\alpha} + \sum_{n'} G^<_{m,n'} V_{n',k\alpha} g^a_{k\alpha} \tag{49}$$

For compactness, we define the following quantities,

$$\sum_{k\alpha}\partial_\mu V_{n,k\alpha}g^r_{k\alpha}V_{k\alpha,m}=\bar{\Sigma}^R_{\mu,nm} \tag{50}$$

$$\sum_{k\alpha}V_{n,k\alpha}g^r_{k\alpha}\partial_\mu V_{k\alpha,m}=\tilde{\Sigma}^R_{\mu,nm} \tag{51}$$

$$\sum_{k\alpha}V_{n,k\alpha}g^a_{k\alpha}\partial_\mu V_{k\alpha,m}=\tilde{\Sigma}^A_{\mu,nm} \tag{52}$$

$$\sum_{k\alpha}\partial_\mu V_{n,k\alpha}g^a_{k\alpha}V_{k\alpha,m}=\bar{\Sigma}^A_{\mu,nm} \tag{53}$$

$$\sum_{k\alpha}V_{n,k\alpha}g^<_{k\alpha}\partial_\mu V_{k\alpha,m}=\tilde{\Sigma}^<_{\mu,nm} \tag{54}$$

$$\sum_{k\alpha}\partial_\mu V_{n,k\alpha}g^<_{k\alpha}V_{k\alpha,m}=\bar{\Sigma}^<_{\mu,nm} \tag{55}$$

$$\sum_{k\alpha}\partial_\nu V_{m,k\alpha}g^<_{k\alpha}\partial_\mu V_{n,k\alpha}=\Sigma^<_{\nu\mu,mn} \tag{56}$$

We then proceed to evaluate Eqs. 37-44. For simplicity, we will apply the wide-band approximation, such that the above quantities are independent of energy ($\epsilon$).

$$\sum_{mnm',k\alpha}\partial_\mu h_{mn}\partial_\epsilon G^R_{nm'}\partial_\nu V_{m',k\alpha}G^<_{k\alpha,m}=\sum_{mnm'n'}\partial_\mu h_{mn}\partial_\epsilon G^R_{nm'}\bar{\Sigma}^<_{\nu,m',n'}G^A_{n',m} \tag{57}$$

$$+\sum_{mnm'n'}\partial_\mu h_{mn}\partial_\epsilon G^R_{nm'}\bar{\Sigma}^R_{\nu,m',n'}G^<_{n',m} \tag{58}$$

$$\sum_{mnm',k\alpha}\partial_\mu h_{mn}\partial_\epsilon G^R_{n,k\alpha}\partial_\nu V_{k\alpha,m'}G^<_{m',m}=\sum_{mnm',n'}\partial_\mu h_{mn}\partial_\epsilon G^R_{n,n'}\tilde{\Sigma}^R_{\nu,n'm'}G^<_{m',m} \tag{59}$$

$$\sum_{mnm',k\alpha}\partial_\mu V_{m,k\alpha}\partial_\epsilon G^R_{k\alpha,m'}\partial_\nu h_{m',n}G^<_{n,m}=\sum_{mnm'n'}\bar{\Sigma}^R_{\mu,mn'}\partial_\epsilon G^R_{n',m'}\partial_\nu h_{m',n}G^<_{n,m} \tag{60}$$

$$\sum_{mnm',k\alpha}\partial_\mu V_{k\alpha,n}\partial_\epsilon G^R_{n,m'}\partial_\nu h_{m',m}G^<_{m,k\alpha}=\sum_{mnm'n'}\tilde{\Sigma}^<_{\mu,n'n}\partial_\epsilon G^R_{n,m'}\partial_\nu h_{m',m}G^R_{m,n'} \tag{61}$$

$$+\sum_{mnm'n'}\tilde{\Sigma}^A_{\mu,n'n}\partial_\epsilon G^R_{n,m'}\partial_\nu h_{m',m}G^<_{m,n'} \tag{62}$$

$$\sum_{mn,k'\alpha',k\alpha}\partial_\mu V_{k\alpha,n}\partial_\epsilon G^R_{n,k'\alpha'}\partial_\nu V_{k'\alpha',m}G^<_{m,k\alpha}=\sum_{mnm'n'}\tilde{\Sigma}^<_{\mu,n'n}\partial_\epsilon G^R_{n,m'}\tilde{\Sigma}^R_{\nu,m'm}G^R_{m,n'} \tag{63}$$

$$+\sum_{mnm'n'}\tilde{\Sigma}^A_{\mu,n'n}\partial_\epsilon G^R_{n,m'}\tilde{\Sigma}^R_{\nu,m'm}G^<_{m,n'} \tag{64}$$

$$\sum_{mn,k'\alpha',k\alpha}\partial_\mu V_{k\alpha,n}\partial_\epsilon G^R_{nm}\partial_\nu V_{m,k'\alpha'}G^<_{k'\alpha',k\alpha}=\sum_{mn}\partial_\epsilon G^R_{nm}\Sigma^<_{\nu\mu,mn} \tag{65}$$

$$+\sum_{mn,n'm'}\tilde{\Sigma}^A_{\mu,m'n}\partial_\epsilon G^R_{nm}\bar{\Sigma}^<_{\nu,mn'}G^A_{n',m'} \tag{66}$$

$$+\sum_{mn,n'm'}\tilde{\Sigma}^A_{\mu,m'n}\partial_\epsilon G^R_{nm}\bar{\Sigma}^R_{\nu,mn'}G^<_{n',m'} \tag{67}$$

$$+\sum_{mn,n'm'}\tilde{\Sigma}^<_{\mu,m'n}\partial_\epsilon G^R_{nm}\bar{\Sigma}^R_{\nu,mn'}G^R_{n',m'} \tag{68}$$

$$\sum_{mn,k'\alpha',k\alpha} \partial_\mu V_{n,k\alpha} \partial_\epsilon G^R_{k\alpha,m} \partial_\nu V_{m,k'\alpha'} G^<_{k'\alpha',n} = \sum_{mn,n',m'} \bar{\Sigma}^R_{\mu,nm'} \partial_\epsilon G^R_{m',m} \bar{\Sigma}^R_{\nu,mn'} G^<_{n',n} \tag{69}$$

$$+ \sum_{mn,n',m'} \bar{\Sigma}^R_{\mu,nm'} \partial_\epsilon G^R_{m',m} \bar{\Sigma}^<_{\nu,mn'} G^A_{n',n} \tag{70}$$

$$\sum_{mn,k'\alpha',k\alpha} \partial_\mu V_{n,k\alpha}, \partial_\epsilon G^R_{k\alpha,k'\alpha'} \partial_\nu V_{k'\alpha',m} G^<_{m,n} = \sum_{mn,m',n'} \Sigma^R_{\mu,nm'} \partial_\epsilon G^R_{m',n'} \tilde{\Sigma}^R_{\nu,n'm} G^<_{m,n} \tag{71}$$

Now Eq. 36-Eq. 44 can be written down as

$$
\begin{aligned}
& Tr_m\left(\partial_\mu \mathcal{H} \partial_\epsilon G^R(\epsilon) \partial_\nu \mathcal{H} G^<(\epsilon)\right) && (72)\\
= \;& Tr_s(\partial_\mu h \partial_\epsilon G^R \partial_\nu h G^<) && (73)\\
+ \;& Tr_s(\partial_\mu h \partial_\epsilon G^R \bar{\Sigma}^<_\nu G^A) && (74)\\
+ \;& Tr_s(\partial_\mu h \partial_\epsilon G^R \bar{\Sigma}^R_\nu G^<) && (75)\\
+ \;& Tr_s(\partial_\mu h \partial_\epsilon G^R \tilde{\Sigma}^R_\nu G^<) && (76)\\
+ \;& Tr_s(\bar{\Sigma}^R_\mu \partial_\epsilon G^R \partial_\nu h G^<) && (77)\\
+ \;& Tr_s(\tilde{\Sigma}^<_\mu \partial_\epsilon G^R \partial_\nu h G^R) && (78)\\
+ \;& Tr_s(\tilde{\Sigma}^A_\mu \partial_\epsilon G^R \partial_\nu h G^<) && (79)\\
+ \;& Tr_s(\tilde{\Sigma}^<_\mu \partial_\epsilon G^R \tilde{\Sigma}^R_\nu G^R) && (80)\\
+ \;& Tr_s(\tilde{\Sigma}^A_\mu \partial_\epsilon G^R \tilde{\Sigma}^R_\nu G^<) && (81)\\
+ \;& Tr_s(\partial_\epsilon G^R \Sigma^<_{\nu,\mu}) && (82)\\
+ \;& Tr_s(\tilde{\Sigma}^A_\mu \partial_\epsilon G^R \bar{\Sigma}^<_\nu G^A) && (83)\\
+ \;& Tr_s(\tilde{\Sigma}^A_\mu \partial_\epsilon G^R \bar{\Sigma}^R_\nu G^<) && (84)\\
+ \;& Tr_s(\tilde{\Sigma}^<_\mu \partial_\epsilon G^R \bar{\Sigma}^R_\nu G^R) && (85)\\
+ \;& Tr_s(\bar{\Sigma}^R_\mu \partial_\epsilon G^R \bar{\Sigma}^R_\nu G^<) && (86)\\
+ \;& Tr_s(\bar{\Sigma}^R_\mu \partial_\epsilon G^R \bar{\Sigma}^<_\nu G^A) && (87)\\
+ \;& Tr_s(\bar{\Sigma}^R_\mu \partial_\epsilon G^R \tilde{\Sigma}^R_\nu G^<) && (88)
\end{aligned}
$$

$Tr_s$ implies summation over system orbitals ($m$ and $n$). The above equations can be further simplified as

$$
\begin{aligned}
& Tr_m\left(\partial_\mu \mathcal{H} \partial_\epsilon \mathcal{G}^R \partial_\nu \mathcal{H} \mathcal{G}^<\right) \\
= \;& Tr_s\left((\partial_\mu h \partial_\epsilon G^R + \bar{\Sigma}^R_\mu \partial_\epsilon G^R + \tilde{\Sigma}^A_\mu \partial_\epsilon G^R)(\partial_\nu h G^< + \partial_\nu \Sigma^R G^< + \bar{\Sigma}^<_\nu G^A)\right) \\
+ \;& Tr_s(\tilde{\Sigma}^<_\mu \partial_\epsilon G^R (\partial_\nu h + \partial_\nu \Sigma^R) G^R + \partial_\epsilon G^R \Sigma^<_{\nu,\mu}) && (89)
\end{aligned}
$$

This is the result presented in the main body of the article. With this result, we can evaluate the non-Condon electronic friction explicitly.
